# Supplementary material for: The Many Faces of Optimal Weak-to-Strong Learning
Source: arXiv:2408.17148 source file (2024-08-30)
Supplement: Supplementary file 1 [file appendixtheoryarxiv.tex]

\section{Proof of \texorpdfstring{\cref{lem15}}{Lg}}
\label{sec:lem4}
We now give the proof of \cref{lem15}.
\ For this we need the following \cref{cor1} that gives and high probability bound on the error for any classifier in $\Dh$ simultaneously that on a sample $S$ has $\gamma$ margins i.e.\ the bound also holds for a $\gamma$-margin classifier algorithm with output in $\Dh$.
\begin{restatable}{corollary}{corollaryone}\label{cor1}
Let $C>1$ denote a universal constant. For hypothesis set $\h$ with VC-dimension $d$, distribution $\dd$, margin $0<\gamma\leq 1$, failure probability  $0<\delta<1$, and a point set $S$ of size $m$ consisting of i.i.d.\ points from $\dd$ we have with probability at least $1-\delta$ over $S$ that any $f\in\Dh$ such that $f(x)c(x)\geq \gamma$ for all $x\in S$:
\begin{align*}
\ld(f) \leq \sqrt{\frac{2Cd}{\gamma^2 m}}+ \sqrt{\frac{2\ln \left(2/\delta\right)}{m}}.
\end{align*}
\end{restatable}
\cref{cor1} follows by a modification of \cite{boostingbook}[page 107-111]  using the stronger bound on the rademacher complexity of $O(\sqrt{d/m})$ due to \cite{Tightvcdudley}[See e.g. theorem 7.2 \cite{rademacherboundlecturenotes} ].
With \cref{cor1} in place we now  give the proof of \cref{lem15} which we for convinece restate before the giving the proof.
\lemfifteen*
\begin{proof}[Proof of \cref{lem15}] Now if $\p\left[R\right]m\leq d/\gamma^2 $ we have that 
$$\sqrt{\frac{d}{\gamma^2\p\left[R\right]m}}\geq 1,$$ 
and the claim holds since $\err(f_S)$ is always less than $1$.
Thus we assume from now on that $\p\left[R\right]m> d/\gamma^2 $. 
We now define the events $E_i:=\{|\{ S\cap R \}|=i\}$ for $m\ge i\geq \p\left[R\right]m /2$  and 
$E=\cup_{i\geq \p\left[R\right]m /2}E_i=\{ |S\cap R|\geq \p\left[R\right]m/2 \}$. We further define $X_j=1\{ S_j\in R \}$ for $j=1,\ldots,m$ and notice that these are i.i.d.\ $\{ 0,1 \}$-random variables where $X=\sum_{j} X_j$ has expectation $\p\left[R\right]m$ and the event $\sum_{j}X_j\geq\p\left[R\right]m/2$ is contained in $E$. Thus by Chernoffs inequality and that $\exp(-x)\leq 1/x$ for $x\geq 0$  we get that 
\begin{align*}
 \p_{S}\left[E\right]\geq 1-\exp\left(-\p\left[R\right]m/8\right)
 \geq 1-\frac{8}{\p\left[R\right]m} 
, \end{align*}
this implies that $\p_{S}\left[\bar{E}\right]\leq 8/\left(\p\left[R\right]m\right)$ which since we assumed that $\p\left[R\right]m\geq d/\gamma^2\geq 1$ and $0\leq x\leq \sqrt{x}$ for $x\leq 1$ further implies that 
\begin{align*}
\p_{S}\left[\bar{E}\right]\leq 8\sqrt{\frac{d}{\gamma^2\p\left[R\right]m}}.
\end{align*}
We will soon show that $\E_{S}\left[\err(f_S)|E_i\right]\leq 22\sqrt{\tfrac{16C d}{\gamma^2\p\left[R\right]m}}$ for $m\geq i\geq \p\left[R\right]m/2$ for a universal constant $C\geq 1$. Now using these 2 relations combined with the law of conditional expectation on the partition $\bar{E}, E_{\p\left[R\right]m/2},\ldots, E_{m}$ and that $\err\leq 1$ we get that
\begin{align*}
\E_{S}\left[\err(f_S)\right]&= \sum_{i\geq p\left[R\right]m/2}\E_{S}\left[\err(f_S)|E_i\right]\p_{S}\left[E_i\right]+\E_{S}\left[\err(f_S)|\bar{E}\right]\p_{S}\left[\bar{E}\right]\\
&\le 22\sqrt{\frac{16C d}{\gamma^2\p\left[R\right]m}}\p\left[E\right] +8\sqrt{\frac{d}{\gamma^2\p\left[R\right]m}}\\
&\leq 30\sqrt{\frac{16C d}{\gamma^2\p\left[R\right]m}}
,\end{align*}
as claimed in \cref{lem15} with the universal constant $a=30^{2}\cdot 16 C$. 
Thus we have to show that $\E_{S}\left[\err(f_S)|E_i\right]\leq 2\sqrt{\tfrac{16C d}{\gamma^2\p\left[R\right]m}}$ for $m\geq i\geq \p\left[R\right]m/2$. So consider such and $i$.
Since $\err(f_S)$ is a non-negative random variable we have that 
\begin{align*}
\E_{S}\left[\err(f_S)\mid E_{i}\right]=\int_{0}^{\infty} \p_{S}\left[\err(f_S)\geq x\mid E_{i}\right] dx
\end{align*}
Thus it is equivalent to showing that the right-hand side is less than the claimed upper bound of $\E_{S}\left[\err(f_S)|E_i\right]$, so we will establish this upper bound instead.
Now conditioned on $E_i$ we know that $S$ contains $i$ points that are samples according to $\dr$ and that $f_S$ on these examples has margin at least $\gamma$. Thus we have by \cref{cor1} that with probability at least $1-\delta$ over $S$ that
\begin{align}\label{lem15:eq1}
  \err(f_S) \leq \sqrt{\max\left(\frac{8Cd}{\gamma^2 i},\frac{8\ln \left(2/\delta\right)}{i}\right)}\end{align}
where $C\geq 1$ is a universal constant. 
For ease of notation let $r_i=\sqrt{\tfrac{8C d}{\gamma^2i}}$ (the left value of the $\max$ in \cref{lem15:eq1}). We notice that $r_i\leq \sqrt{\tfrac{16C d}{\gamma^2\p\left[R\right]m}}$ since $i$ is assumed to be gerater than $\p\left[R\right]m/2$. Using this we get that
\begin{align}\label{lem15:eq3}
\int_{0}^{\infty} \p_{S}\left[\err(f_S)\geq x\mid E_{i}\right] dx
\leq   r_i\leq \sqrt{\tfrac{16C d}{\gamma^2\p\left[R\right]m}}+\int_{r_{i}}^{\infty} \p_{S}\left[\err(f_S)\geq x\right] dx
.\end{align}
Thus if we can show that
\begin{align*}
\int_{r_{i}}^{\infty} \p_{S}\left[\err(f_S)\geq x\right] dx \leq  21 \sqrt{\tfrac{ d}{\gamma^2\p\left[R\right]m}}
,\end{align*}
we get by combining this with \cref{lem15:eq3} that 
\begin{align*}
  \E_{S}\left[\err(f_S)\mid E_{i}\right] \leq 22 \sqrt{\tfrac{16C d}{\gamma^2\p\left[R\right]m}}
  \end{align*}
with which would conclude the proof. 
Thus we now show $\int_{r_{i}}^{\infty} \p_{S}\left[\err(f_S)\geq x\right] dx\leq 21\sqrt{\frac{d}{\gamma^2\p\left[R\right]m}}$. For this we rewrite $x$ as \begin{align*}
x=\sqrt{8\ln \left(\frac{2}{2\exp \left(\frac{-x^{2}i}{8}\right)}\right)/i}.
\end{align*}
Now for any $x\geq r_i$ we have that 
\begin{align*}
\p_{S}\left[\err(f_S)\geq x)\mid E_{i}\right]=\p_{S}\left[\err(f_S)\geq \max(r_i,x))\mid E_{i}\right]
, \end{align*}
which combined with the rewrite of $x$ and \cref{lem15:eq1} with  $\delta=2\exp \left(\frac{-x^{2}i}{8}\right)$ and noticing $r_i$ is the left value in $\max$ of \cref{lem15:eq1}, we get that 
 \begin{align*}
\p_{S}\left[\err(f_S)\geq x\mid E_{i}\right]=\p_{S}\left[\err(f_S)\geq \max(r_i,x)\mid E_{i}\right]\leq 2\exp \left(\frac{-x^{2}i}{8}\right), \end{align*}
for any $x\geq r_i$.
Now using the density function of a normal distribution with mean $0$ and standard deviation $\sigma$ is equal to $1/(\sigma\sqrt{2\pi})\exp(-\frac{1}{2}(x/\sigma)^2)$, and letting $N(0,\sigma)$ denote a normal random variable with mean $0$ and standard deviation $\sigma$ we get that
\begin{align*}
&\int_{r_{i}}^{\infty} \p_{S}\left[\err(f_S)\geq x\mid E_i\right] dx\leq \int_{r_{i}}^{\infty}2\exp \left(\frac{-x^{2}i}{8}\right) dx
\\
&\leq 2\sqrt{8/(2i)}\sqrt{2\pi}\int_{r_{i}}^{\infty} \frac{1}{\sqrt{8/(2i)}\sqrt{2\pi}}\exp \left(-\frac{1}{2}\left(\frac{x^{2}}{\sqrt{8/(2i)}}\right)^2\right) dx\\
&\leq 2\sqrt{(8/(2i))}\sqrt{2\pi}\p\left[N\left (0,\sqrt{ \frac{8}{2i}}\right )\geq r_i\right]
\leq 8\sqrt{\pi}\sqrt{2/\p\left[R\right]m}\leq 21\sqrt{\frac{d}{\gamma^2\p\left[R\right]m}}
,\end{align*}
where the second to last inequality follows from $i\geq \p\left[R\right]m/2$ and the last inequality by $\p\left[R\right]m\geq d/\gamma^2\geq 1$.
\end{proof}
